# Supplementary material for: Modeling meteorite craters by impacting melted tin on sand
Source: arXiv:2303.18016 source file (2023-03-31)
Supplement: Supplementary file 1 [file Scientific_Report_SI.pdf]

# Modeling meteorite craters by impacting melted tin on sand

**H. Y. Huang[1], P. R. Tsai[1], C. Y. Lu[1], H. Hau[1], Y. L. Chen[2], Z. T. Ling[3], Y. R. Wu[4], and Tzay-Ming Hong[1,*]**

[1]Department of Physics, National Tsing Hua University, Hsinchu, Taiwan 30013, Republic of China
[2]Department of Mechanical Engineering, National Taiwan University, Taipei, Taiwan 10617, Republic of China
[3]Department of New Media Art, Taipei National University of the Arts, Taipei, Taiwan 110024, Republic of China
[4]National Hsinchu Senior High School, Hsinchu, Taiwan 30013, Republic of China
[*]ming@phys.nthu.edu.tw

## ABSTRACT

## Mapping raw files to network systems

Throughout the analysis of melted tin images using graph theory, we will divide them into four main steps:

### Methods: Texture Segmentation Using Gabor Filters

For the image segmentation of tin and granules, image preprocessing can help us reduce the interference from granules with the subsequent analysis[1]. With Gabor filters, we can perform information extraction from raw files. Gabor filter operates similarly to the simple cells in the visual area V1 of the brain for line extraction of image texture. It performs extraction in different polarized directions to retain important contours[2]. Since granules and tin have different textures, there must be different residual information in Gabor filter extraction. Therefore, we can carry out population grouping on this information based on statistical characteristics. Here, we use K-means clustering with Replicates=5 and centers=2 to process images with a resolution of 256×256 so as to distinguish granules and tin ball, as shown in Fig. 1.

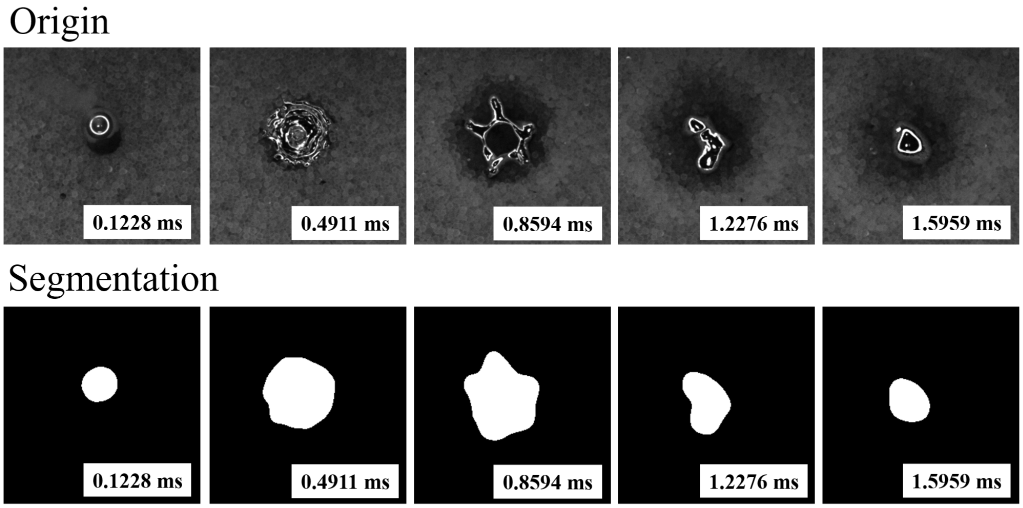


**Figure 1.** Texture segmentation for snapshots shows the evolution of melted tin with $R = 6.4$ mm, 380 °C and $h = 50$ mm.

## Methods: Convolutional Neural Network (CNN)

We can construct a classifier using CNN[3] to label the shape of tin remnant obtained from texture segmentation. CNN is a deep learning network with the ability to extract features from images. Inspired by the response process of the visual system in the brain to incoming image information, CNN also exhibits translational invariance in detecting image information.

We can classify different shapes of tin remnant according to images that have undergone texture segmentation, and use CNN for supervised learning with known answers. Employing 5000 samples for each shape, we adjust the Training-Validation rate to 6:4, MiniBatchSize=128, MaxEpochs=10, LearnRate=$10^{-4}$. The network structure and learning curves are shown in Figs. 2 and 3, respectively.

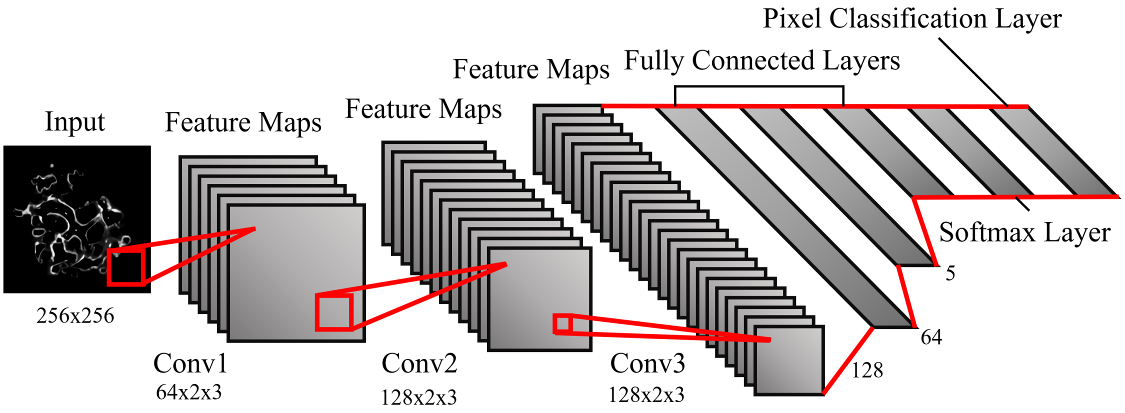


**Figure 2.** Network structure of CNN

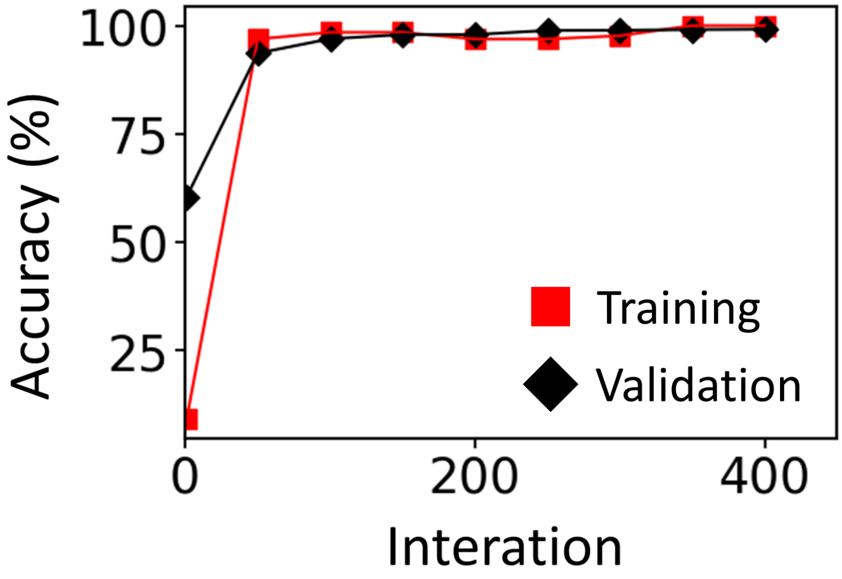


**Figure 3.** Learning curves for training and validation accuracy

## Methods: Grad-CAM

To develop a better comprehension of how deep learning functions with stimuli, we employ visualization techniques, such as gradient-weighted class activation mapping (Grad-CAM)[4]. The Grad-CAM method utilizes information from the soft-max layer to generate feature maps $A_{kij}$ for an image, where $k$ represents the label of the feature map, and $i$ and $j$ denote the spatial resolution. By performing backpropagation, we can calculate the gradient of the score with respect to the feature maps, which

are treated as a weight $W(k)$. Subsequently, we apply ReLU linear combination $L_{\text{Grad-CAM}} = \text{ReLU}(W(k)A_k)$ to the image and perform upsampling to generate a Grad-CAM image.

In our study, we utilize Grad-CAM to capture the locations of features that CNN uses to identify different shapes of tin remnant in photographs. This allowed us to extract important information of tin.

### Methods: Graph Density and Average Length

Graph theory is an effective mathematical tool for establishing and analyzing relationships in groups and is widely used in various fields, such as physics for phase transition problems, sociology for urban planning, and neuroscience for brain response. We will scale down the two-dimensional Grad-CAM scoring results from $256\times256$ to $32\times32$, and normalize the scaled scores. Afterward, 20% of the normalized scores are used as the threshold to eliminate unimportant parts, and then binarize the pixels with values and without values, using a value of "1" as the standard for node construction. To define shapes based on the scattered state of tin remnant, we set $d(i,j)$ as the distance between nodes and calculate the average distance $L \equiv [2\sum_{i,j=1}^{N} d(i,j)]/[N(N-1)]$ as the condition for link establishment. If $d(i,j) \geq L$, a link is formed. This is to ensure that the lowest standard for edge establishment is maintained between group nodes. Finally, we calculate graph density $D \equiv E/[V(V-1)]$ where $E$ is the number of links and $V$ is the number of nodes to represent the differences between shapes, achieving a numerical definition of shapes under the network structure.

## Why melted tin dug a deeper crater than steel ball?

The obvious difference from steel ball is that melted tin can deform. Armed with a high-speed camera, we can determine the shape of melted tin in stage 2, whose center of mass and depth $d_c$ are subsequently calculated. Although melted tin eventually dug a deeper crater in stage 4 as shown in Fig. 5(b, d) of the main text, its $d_c$ is roughly the same as that of steel ball with the same mass and impact energy. How is this possible? The key turns out to be that melted tin in its liquid phase can deform and extend vertically to carve out a deeper hole, as shown schematically in Fig. 4. This explanation is consistent with the fact that the discrepancy of $d$ for melted tin and steer ball increases with temperature.

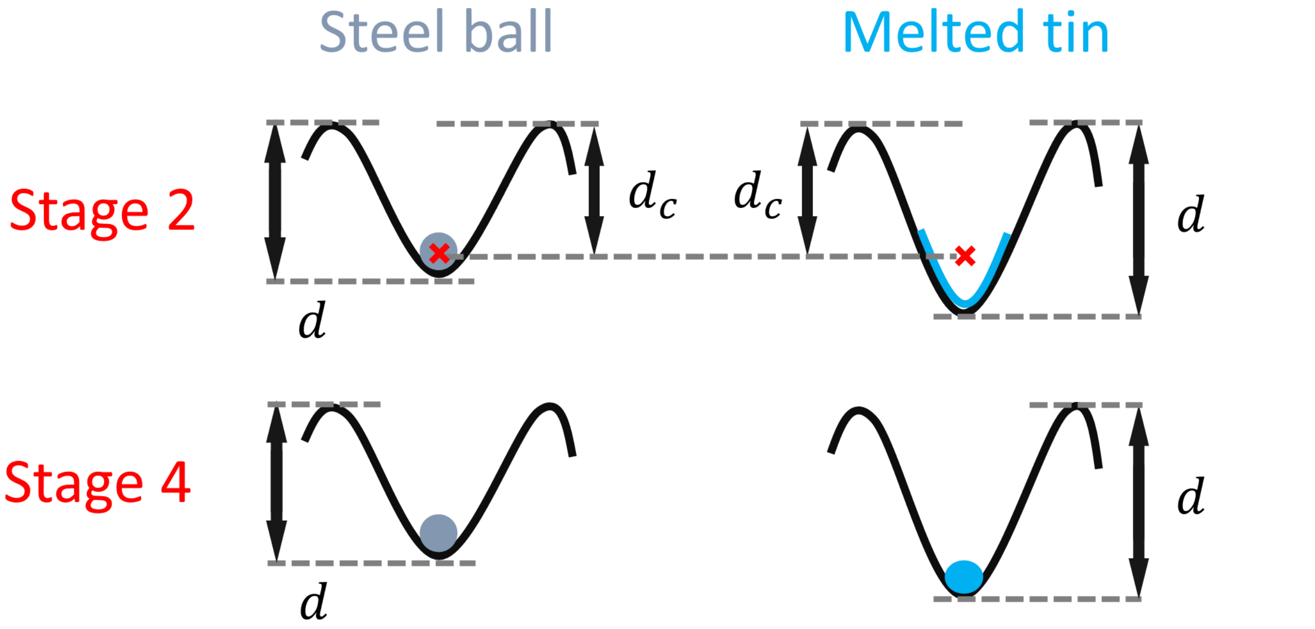


**Figure 4.** Schematic profiles of tin and crater in stages 2 and 4 where the red cross indicates the position of center of mass.

## References

**1.** Jain, Anil K, and Farshid Farrokhnia, Unsupervised texture segmentation using Gabor filters, Pattern recognition **24**, 1167-1186 (1991).

**2.** Jones, Judson P, Aaron Stepnoski, and Larry A. Palmer, The two-dimensional spectral structure of simple receptive fields in cat striate cortex, Journal of Neurophysiology, **58**, 1212-1232 (1987).

**3.** Li, Zewen, et al, A survey of convolutional neural networks: analysis, applications, and prospects, IEEE transactions on neural networks and learning systems (2021).

**4.** Selvaraju, Ramprasaath R, et al, Grad-cam: Visual explanations from deep networks via gradient-based localization. Proceedings of the IEEE international conference on computer vision. (2017).
